# Supplementary material for: Learning to Sample
Source: arXiv:1812.01659 source file (2019-04-01)
Supplement: Supplementary file 1 [file main_supplementary.tex]

% \documentclass[10pt,twocolumn,letterpaper]{article}

% \usepackage{cvpr}
% \usepackage{times}
% \usepackage{epsfig}
% \usepackage{graphicx}
% \usepackage{amsmath}
% \usepackage{amssymb}

% % Include other packages here, before hyperref.

% % If you comment hyperref and then uncomment it, you should delete
% % egpaper.aux before re-running latex.  (Or just hit 'q' on the first latex
% % run, let it finish, and you should be clear).
% \usepackage[pagebackref=true,breaklinks=true,letterpaper=true,colorlinks,bookmarks=false]{hyperref}

% % \cvprfinalcopy % *** Uncomment this line for the final submission

% \def\cvprPaperID{1910} % *** Enter the CVPR Paper ID here
% \def\httilde{\mbox{\tt\raisebox{-.5ex}{\symbol{126}}}}

% \newcommand{\SNET}{S-NET }
% \newcommand{\SNETwo}{S-NET}

% % Pages are numbered in submission mode, and unnumbered in camera-ready
% \ifcvprfinal\pagestyle{empty}\fi
% \begin{document}

% %%%%%%%%% TITLE
% \title{Learning to Sample - Supplementary Material}

% \author{First Author\\
% Institution1\\
% Institution1 address\\
% {\tt\small firstauthor@i1.org}
% % For a paper whose authors are all at the same institution,
% % omit the following lines up until the closing ``}''.
% % Additional authors and addresses can be added with ``\and'',
% % just like the second author.
% % To save space, use either the email address or home page, not both
% \and
% Second Author\\
% Institution2\\
% First line of institution2 address\\
% {\tt\small secondauthor@i2.org}
% }

% \maketitle
% %\thispagestyle{empty}

% %%%%%%%%% EXPERIMENTAL DETAILS
% %-------------------------------------------------------------------------
% \section{Experimental details}
% \input{supplementary/experimental_details}

% \section{Regularization}
% \input{supplementary/regularization}

% \section{Critical set sampling}
% \input{supplementary/critical_set.tex}

% \section{Reconstruction}
% \input{supplementary/reconstruction.tex}

% %%%%%%%%% REFERENCES
% %-------------------------------------------------------------------------
% {\small
% % \bibliographystyle{ieee}
% \bibliographystyle{IEEEtran}
% \bibliography{IEEEabrv,references}
% }

% \end{document}
