# Supplementary material for: Learning to Sample
Source: arXiv:1812.01659 source file (2019-04-01)
Supplement: Supplementary file 2 [file progressive_sampling.tex]

% %---------------------------------------             Progressive Sampling
% \begin{figure*}[h]
% \begin{center}
% \begin{tabular}{ c c c c c }
% Input $2048$ & ProgressiveNet $32$ & ProgressiveNet $64$ & ProgressiveNet $128$ & ProgressiveNet $256$ \\
% \includegraphics[width=0.17\linewidth]{supplementary/Images/reconstruction/car_295_progressivenet_multi_samp_fps_2048_crop} &
% \includegraphics[width=0.17\linewidth]{supplementary/Images/reconstruction/car_295_progressivenet_multi_samp_prj_0032_crop} &
% \includegraphics[width=0.17\linewidth]{supplementary/Images/reconstruction/car_295_progressivenet_multi_samp_prj_0064_crop} &
% \includegraphics[width=0.17\linewidth]{supplementary/Images/reconstruction/car_295_progressivenet_multi_samp_prj_0128_crop} &
% \includegraphics[width=0.17\linewidth]{supplementary/Images/reconstruction/car_295_progressivenet_multi_samp_prj_0256_crop} \\

% \includegraphics[width=0.17\linewidth]{supplementary/Images/reconstruction/car_295_progressivenet_multi_rcon_fps_2048_crop} &
% \includegraphics[width=0.17\linewidth]{supplementary/Images/reconstruction/car_295_progressivenet_multi_rcon_prj_0032_crop} &
% \includegraphics[width=0.17\linewidth]{supplementary/Images/reconstruction/car_295_progressivenet_multi_rcon_prj_0064_crop} &
% \includegraphics[width=0.17\linewidth]{supplementary/Images/reconstruction/car_295_progressivenet_multi_rcon_prj_0128_crop} &
% \includegraphics[width=0.17\linewidth]{supplementary/Images/reconstruction/car_295_progressivenet_multi_rcon_prj_0256_crop} \\

% Input $2048$ & FPS $32$ & FPS $64$ & FPS $128$ & FPS $256$ \\
% \includegraphics[width=0.17\linewidth]{supplementary/Images/reconstruction/car_295_progressivenet_multi_samp_fps_2048_crop} &
% \includegraphics[width=0.17\linewidth]{supplementary/Images/reconstruction/car_295_progressivenet_multi_samp_fps_0032_crop} &
% \includegraphics[width=0.17\linewidth]{supplementary/Images/reconstruction/car_295_progressivenet_multi_samp_fps_0064_crop} &
% \includegraphics[width=0.17\linewidth]{supplementary/Images/reconstruction/car_295_progressivenet_multi_samp_fps_0128_crop} &
% \includegraphics[width=0.17\linewidth]{supplementary/Images/reconstruction/car_295_progressivenet_multi_samp_fps_0256_crop} \\

% \includegraphics[width=0.17\linewidth]{supplementary/Images/reconstruction/car_295_progressivenet_multi_rcon_fps_2048_crop} &
% \includegraphics[width=0.17\linewidth]{supplementary/Images/reconstruction/car_295_progressivenet_multi_rcon_fps_0032_crop} &
% \includegraphics[width=0.17\linewidth]{supplementary/Images/reconstruction/car_295_progressivenet_multi_rcon_fps_0064_crop} &
% \includegraphics[width=0.17\linewidth]{supplementary/Images/reconstruction/car_295_progressivenet_multi_rcon_fps_0128_crop} &
% \includegraphics[width=0.17\linewidth]{supplementary/Images/reconstruction/car_295_progressivenet_multi_rcon_fps_0256_crop} \\

% \end{tabular}
% \caption{{\bfseries Progressive sampling.} First and third rows: Input point cloud and samples of different sizes of ProgressiveNet and FPS, respectively. Second and fourth rows: reconstruction from the input point cloud and from the corresponding samples. The sampled points are enlarged for visualization purpose. Even at a low sample size as 64 points, the reconstruction from ProgressiveNet's points is visually similar to the reconstruction from the complete input point cloud. On the contrary, it takes four times more FPS points to achieve this level of similarity.}
% \label{fig:progressive_sampling}
% \end{center}
% \end{figure*}

% Figure~\ref{fig:progressive_sampling} presents a visual example of the points sampled by ProgressiveNet and by FPS, for various sample sizes, along with their corresponding reconstructions. The complete input point cloud and its reconstruction are shown as well. The shape was taken from the test split of the data.

% % ProgressiveNet orders the points such that even with only 64 points, the reconstruction resembles the reconstruction from the complete 2048 point set. FPS is agnostic to the reconstruction task. Thus, when sampling the same number of points, it results in an inferior reconstruction. When the number of sampled points is increased towards 256 points, the reconstructions from both sampling methods becomes similar. The reader is also referred to the attached video, showing a step by step example of progressive sampling.

% % \begin{figure*}
% % \begin{center}
% % \begin{tabular}{ c c c c c }
% % Input $2048$ & ProgressiveNet $32$ & FPS $32$ & ProgressiveNet $64$ & FPS $64$ \\
% % \includegraphics[width=0.17\linewidth]{supplementary/Images/reconstruction/car_295_progressivenet_multi_samp_fps_2048_crop} &
% % \includegraphics[width=0.17\linewidth]{supplementary/Images/reconstruction/car_295_progressivenet_multi_samp_prj_0032_crop} &
% % \includegraphics[width=0.17\linewidth]{supplementary/Images/reconstruction/car_295_progressivenet_multi_samp_fps_0032_crop} &
% % \includegraphics[width=0.17\linewidth]{supplementary/Images/reconstruction/car_295_progressivenet_multi_samp_prj_0064_crop} &
% % \includegraphics[width=0.17\linewidth]{supplementary/Images/reconstruction/car_295_progressivenet_multi_samp_fps_0064_crop} \\

% % \includegraphics[width=0.17\linewidth]{supplementary/Images/reconstruction/car_295_progressivenet_multi_rcon_fps_2048_crop} &
% % \includegraphics[width=0.17\linewidth]{supplementary/Images/reconstruction/car_295_progressivenet_multi_rcon_prj_0032_crop} &
% % \includegraphics[width=0.17\linewidth]{supplementary/Images/reconstruction/car_295_progressivenet_multi_rcon_fps_0032_crop} &
% % \includegraphics[width=0.17\linewidth]{supplementary/Images/reconstruction/car_295_progressivenet_multi_rcon_prj_0064_crop} &
% % \includegraphics[width=0.17\linewidth]{supplementary/Images/reconstruction/car_295_progressivenet_multi_rcon_fps_0064_crop} \\

% % Input $2048$ & ProgressiveNet $128$ & FPS $128$ & ProgressiveNet $256$ & FPS $256$ \\
% % \includegraphics[width=0.17\linewidth]{supplementary/Images/reconstruction/car_295_progressivenet_multi_samp_fps_2048_crop} &
% % \includegraphics[width=0.17\linewidth]{supplementary/Images/reconstruction/car_295_progressivenet_multi_samp_prj_0128_crop} &
% % \includegraphics[width=0.17\linewidth]{supplementary/Images/reconstruction/car_295_progressivenet_multi_samp_fps_0128_crop} &
% % \includegraphics[width=0.17\linewidth]{supplementary/Images/reconstruction/car_295_progressivenet_multi_samp_prj_0256_crop} &
% % \includegraphics[width=0.17\linewidth]{supplementary/Images/reconstruction/car_295_progressivenet_multi_samp_fps_0256_crop} \\

% % \includegraphics[width=0.17\linewidth]{supplementary/Images/reconstruction/car_295_progressivenet_multi_rcon_fps_2048_crop} &
% % \includegraphics[width=0.17\linewidth]{supplementary/Images/reconstruction/car_295_progressivenet_multi_rcon_prj_0128_crop} &
% % \includegraphics[width=0.17\linewidth]{supplementary/Images/reconstruction/car_295_progressivenet_multi_rcon_fps_0128_crop} &
% % \includegraphics[width=0.17\linewidth]{supplementary/Images/reconstruction/car_295_progressivenet_multi_rcon_prj_0256_crop} &
% % \includegraphics[width=0.17\linewidth]{supplementary/Images/reconstruction/car_295_progressivenet_multi_rcon_fps_0256_crop} \\

% % \end{tabular}
% % \caption{{\bfseries Progressive sampling.} First and third rows: Input point cloud and samples of different size of ProgressiveNet and FPS. Second and fourth rows: reconstruction from the input point cloud and form corresponding samples. The sampled points are enlarged for visualization purpose. Even at a low sample size as 64 points, the reconstruction from ProgressiveNet's points is visually similar to the reconstruction from the complete input point cloud. On the contrary, it takes four times more FPS points to achieve this level of similarity.}
% % \label{fig:progressive_sampling}
% % \end{center}
% % \end{figure*}
