# Supplementary material for: Learning to Sample
Source: arXiv:1812.01659 source file (2019-04-01)
Supplement: Supplementary file 3 [file reconstruction.tex]

The number of unique points after forward matching is shown in Figure~\ref{fig:recon_unique_vs_gen_chair}. We can see that the graph grows sub-linearly. This means that as the number of generated points increases, they cover less of the input point cloud, and the FPS completion in the matching process is more dominant.

% \begin{figure}
% \begin{center}
% \includegraphics[width=1.0\linewidth]{supplementary/images/reconstruction/chair_class_norm_loss_vs_samp_ratio_1_64}
% \end{center}
% \caption{Chair-class reconstruction loss vs. normalized reconstruction error (SampleNet and ProgressiveNet).}
% \label{fig:recon_loss_vs_samp_size_chair}
% \end{figure}

% \begin{figure}
% \begin{center}
% \includegraphics[width=1.0\linewidth]{supplementary/images/reconstruction/chair_class_n_unique_vs_n_samp}
% \end{center}
% \caption{Chair class number of unique points vs. number of generated points.}
% \label{fig:recon_unique_vs_gen_chair}
% \end{figure}
