# Supplementary material for: Learning to Sample
Source: arXiv:1812.01659 source file (2019-04-01)
Supplement: Supplementary file 4 [file retrieval.tex]

% Figure~\ref{fig:retrieval_eamples} shows an example of the top 5 retrievals by either S-NET or FPS when using 32 sampled points, as detailed in Section~\ref{sec:retrieval_results}

% \begin{figure*}
% \begin{center}
% \begin{tabular}{ c| c c c c c}
% Query  & \multicolumn{5}{c}{S-NET-32 top five retrieval CAD Models}   \\
% \includegraphics[width=0.14\linewidth]{supplementary/Images/retrieval/plant_0241.png} &
% \includegraphics[width=0.14\linewidth]{supplementary/Images/retrieval/plant_0332.png} &
% \includegraphics[width=0.14\linewidth]{supplementary/Images/retrieval/plant_0288.png} &
% \includegraphics[width=0.14\linewidth]{supplementary/Images/retrieval/plant_0248.png} &
% \includegraphics[width=0.14\linewidth]{supplementary/Images/retrieval/vase_0506.png} &
% \includegraphics[width=0.14\linewidth]{supplementary/Images/retrieval/plant_0244.png} \\
% plant & plant & plant & plant & vase & plant \\
% \hline
% Query  & \multicolumn{5}{c}{FPS-32 top five retrieval CAD Models}   \\
% \includegraphics[width=0.14\linewidth]{supplementary/Images/retrieval/plant_0241.png} &
% \includegraphics[width=0.14\linewidth]{supplementary/Images/retrieval/bowl_0084.png} &
% \includegraphics[width=0.14\linewidth]{supplementary/Images/retrieval/sofa_0776.png} &
% \includegraphics[width=0.14\linewidth]{supplementary/Images/retrieval/sofa_0754.png} &
% \includegraphics[width=0.14\linewidth]{supplementary/Images/retrieval/sofa_0749.png} &
% \includegraphics[width=0.14\linewidth]{supplementary/Images/retrieval/plant_0319.png} \\
% plant & bowl & sofa & sofa & sofa & plant \\

% \end{tabular}
% \caption{{\bfseries Retrieval example.} }
% \label{fig:retrieval_eamples}
% \end{center}
% \end{figure*}
