# Supplementary material for: Learning to Sample
Source: arXiv:1812.01659 source file (2019-04-01)
Supplement: Supplementary file 5 [file sampling_pattern.tex]

We define the radius of a point as $r = \sqrt{x^2+y^2+z^2}$, keeping in mind that of the point clouds in the dataset were normalized to the unit sphere.

\begin{figure}
\includegraphics[width=\columnwidth]{supplementary/Images/radius_by_index.eps}
\caption{{\bfseries Average point radius as function of its index in FPS vs ProgressiveNet ordering.}}
\label{fig:radius_by_index}
\end{figure}

Figure ~\ref{fig:radius_by_index} shows the average point radius as a function of the point order, either by FPS or ProgressiveNet ordering. We see that FPS , other than the first point which is randomly selected, tends to sample points with high radius first (as expected, since they are farthest away from each other). ProgressiveNet learned a very different sampling pattern, where it alternates between sampling points with very high and very low radiuses, i.e, both on the outer boundaries and deep inside the shape. We notice that this sampling pattern emerged when averaging over all of the test set. We would expect that any random pattern will diminish when averaging over the whole test set and therefore we conclude that this sampling pattern is meaningful.
